# Supplementary material for: InfiFusion: A Unified Framework for Enhanced Cross-Model Reasoning via LLM Fusion
Source: arXiv:2501.02795 source file (2025-02-17)
Supplement: Supplementary file 1 [file Appendix.loss.tex]

\section*{Appendix D: Impacts of Losses}
